# Supplementary material for: A Survey of Microarchitectural Side-channel Vulnerabilities, Attacks and Defenses in Cryptography
Source: arXiv:2103.14244 source file (2021-03-26)
Supplement: Supplementary file 1 [file appendix.tex]

\appendix

\subsection{Cryptographic Ciphers and Protocols}
\label{sec:append-crypto}

\subsubsection{Elliptic Curve Cryptography}
\label{sec:append-ecc}
In geometry, an elliptic curve is a two-dimensional curve defined by $y^2 = x^3 + ax + b$.
When used in cryptography, we make a few modifications. We first require $4a^3 + 27b^2 \neq 0$
to exclude singularity. Additionally we apply the curve over a finite field, usually with a prime
or $2^m$ order, and introduce a special infinity point $\infty$. This forms a group of points, 
with $\infty$ as identity element and the $+$ operation defined as: 1) $P+\infty=P$;
2) if $P$ is the reflection of $Q$ over the x-axis, then $P+Q=\infty$; 3) if $P$ and $Q$ are
different points not in case 2, then the line through $P$ and $Q$ intersects the curve
with another point $R$, then $P+Q=R'$ where $R'$ is the reflection of $R$ over the x-axis;
4) if $P$ and $Q$ are the same point, treat ``the line through
$P$ and $Q$'' as ``the line tangent to the curve at $P$'' and use case 3. Case 3 and 4 are non-trivial cases
and can be computed with Equation \ref{eq:pointadd}. We usually write $P+...+P$ as $nP$, and name
this operation ``scalar multiplication''. 
%The security of Elliptic Curve Cryptography is based on the difficulty of Elliptic Curve Discrete Logarithm Problem: given $P$ and $nP$, computing $n$ is hard.

%The set of all points forms a elliptic curve group. The group defines the inverse of a point $P$ as the one symmetric about the x-axis. It also defines the addition operation over two points $P$ and $Q$ in Equation \ref{eq:pointadd}. With such definitions, elliptic curve can be used in cryptography  \cite{Mi:85, Ko:87}.

\begin{align}
\label{eq:pointadd}
\footnotesize
\begin{split}
& \lambda = 
\begin{cases}
    \frac{y_q - y_p}{x_q - x_p}, & \text{if } x_q\neq x_p\\
    \frac{3x^2_p + a}{2y_p},              & \text{otherwise}
\end{cases} \\
&x_r = \lambda^2 - x_p - x_q \\
&y_r = \lambda(x_p - x_r) - y_p
\end{split}
\end{align}

Elliptic curve can be used in cryptography \cite{Mi:85, Ko:87}. Assuming the group has
prime order $p$ and generator $G$, choose a random integer $k$ from $[1, p-1]$ as
the private key, then $D=kG$ will be the public key. 

\bheading{Usage in Digital Signature (ECDSA)}. To sign message $m$, Alice chooses a public
hash function $h$ and a secret nonce $n$. Compute $R = nG \mod p$, $r = R_x$ (cannot be zero),
and $s = k^{-1}(h(m)+kr) \mod p$, then $(r,s)$ is the signature. To verify, Bob computes
$u_1 = h(m)s^{-1} \mod p$, $u_2 = rs^{-1} \mod p$, $Z = u_1G + u_2D$, and $z = Z_x$. The
signature is valid if $r \equiv z \mod p$ holds.

\bheading{Usage in Key Exchange (ECDH)}. Assuming Alice uses private key $k_A$ and public
key $P_A=k_AG$, and Bob similarly uses key pair $(k_B, P_B)$, the shared symmetric key is
simply $k = k_BP_A = k_AP_B = (k_Ak_B)G$.

\subsubsection{Key Exchange and Encryption Protocols}
\label{sec:append-pad}

In the handshake protocol, the client first sends a list of cipher suites $cs_c$ and a nonce $r_c$.
The server responds with a list of cipher suites $cs_s$, the server certificate, and a nonce $r_s$.
Then the client picks a cipher $cs$ (e.g., RSA) supported by both the client and server.

The client generates a random secret string $k$ with byte length $l_k$ as the master key.
We require $l_k \leqslant l_n-11$, where $l_n$ is the byte length of $n$ in the server's
public key $(n, e)$. The client builds a message block $m$ (Equation \ref{eq:rsa}a) using a non-zero
random padding string \texttt{pad} with byte length $l_n - 3 – l_k$, which is at least 8.
Then she encrypts $m$ to get the ciphertext (Equation \ref{eq:rsa}b).

\begin{subequations}
\label{eq:rsa}
\footnotesize
  \begin{align}
& m = 0x00 || 0x02 || \texttt{pad} || 0x00 || k \\
& c \equiv m^e \mod n
  \end{align}
\end{subequations}

The server decrypts the received ciphertext and validates if the message format complies with
Equation \ref{eq:rsa}a. If yes, the server sends a finished message to the client,
and the client replies a finished message, marking the completion of the key exchange of $k$.

Equation \ref{eq:mac-cbc} shows how to use CBC-MAC to encrypt message $m$ with MAC
built from a block cipher of block size $b$. (1) The MAC $HM$ is calculated over
the sequence number \texttt{SEQ}, header \texttt{HDR} and message $m$ (Equation \ref{eq:mac-cbc}a).
(2) The plaintext $P$ is created by concatenating $m$, $HM$, and a padding string
\texttt{pad} (Equation \ref{eq:mac-cbc}b) chosen so that the byte length of P
is $Nb$, where $N$ is an integer. The most common way is to pad $n+1$
bytes with each byte value as $n$, e.g., $0x02||0x02||0x02$. (3)
$P$ is divided into a sequence of blocks of $b$ bytes, $p_1, p_2, ..., p_N$, and encrypted
with key $K$ (Equation \ref{eq:mac-cbc}c). (4) The text $T$ transmitted over the network
is the concatenation of \texttt{HDR} and each ciphertext block (Equation \ref{eq:mac-cbc}d).

\begin{subequations}
\label{eq:mac-cbc}
\footnotesize
\vspace{-4pt}
  \begin{align}
& HM = H((K \oplus \texttt{opad}) || H((K \oplus \texttt{ipad})||\texttt{SEQ} || \texttt{HDR} || m)) \\
& P = m || HM || \texttt{pad} \\
& c_i = Enc_K(c_{i-1} \oplus p_i); i = 1, 2, ..., N \\
& T = \texttt{HDR} || c_1 || c_2 || .. || c_N
  \end{align}
\end{subequations}

The receiver decrypts $T$ and accepts the message $m$ only if the padding format and MAC are correct.

\subsection{Implementations of Cryptographic Operations}
\label{sec:append-implement}

We show the pseudo code of implementations for different cryptographic operations described in
Section \ref{sec:crypto}.

\RestyleAlgo{ruled}
\SetAlgoLined
\LinesNumbered

{\centering
\removelatexerror
\begin{minipage}{\linewidth}
\begin{algorithm}[H]
\scriptsize
\SetAlgoLined
 \KwIn{$x$:$x_{k-1}x_{k-2}...x_0$, $y$:$y_{n-1}y_{n-2}...y_0$}
 \Indp 
\Indm \KwOut{$x*y$}
\Indp
\Indm
\SetKwFunction{proc}{MULTIPLY}
\SetKwProg{myalg}{function}{}{end}
    \BlankLine
    \BlankLine
  \myalg{\proc{$x, y$}}{
  \If{\emph{$\texttt{SIZE\_OF\_LIMBS}(x) < \texttt{KARATSUBA\_THRESHOLD}$}} {
    $r\gets \texttt{MUL\_BASECASE}(x, y)$
  }
  $r \gets 0$ \\
  $i \gets 1$ \\
  \While{$i*n \leq k$}{
    $t \gets \texttt{MUL\_KARATSUBA}(x_{i*n-1}...x_{(i-1)*n}, y)$ \\
    $r \gets \texttt{ADD\_WITH\_OFFSET}(r, t, (i-1)*n)$ \\
    $i \gets i+1$
  }
  \If{$i*n>k$}{
    $t \gets \texttt{MULTIPLY}(b, a_{k-1}...a_{(i-1)*n})$ \\
    $r \gets \texttt{ADD\_WITH\_OFFSET}(r, t, (i-1)*n)$ \\
  }
  \KwRet $r$
}

\SetKwFunction{proc}{MUL\_BASECASE}
\SetKwProg{myalg}{function}{}{end}
    \BlankLine
    \BlankLine
\myalg{\proc{$x, y$}}{
  \uIf{$y_0 = 0$}{
    $r \gets 0$
  }\uElseIf{$y_0 = 1$}{
      $r \gets x$
  }\uElse{
      $r \gets \texttt{MUL\_BY\_SINGLE\_LIMB}(x, y_0)$
  }

  \For{$i \gets 1$ \textbf{\emph{to}} $n-1$ } {
    \uIf{$y_i = 1$}{
      $r \gets \texttt{ADD\_WITH\_OFFSET}(r, x, i)$
    }\uElseIf{$y_i > 1$}{
      $r \gets \texttt{MUL\_AND\_ADD\_WITH\_OFFSET}(r, x, y_i, i)$
    }
  }

  \KwRet $r$
}

\SetKwFunction{proc}{MUL\_KARATSUBA}
\SetKwProg{myalg}{function}{}{end}
    \BlankLine
    \BlankLine
\myalg{\proc{$x, y$}}{
  \If{\emph{$n < \texttt{KARATSUBA\_THRESHOLD}$}}{
    \KwRet $\texttt{MUL\_BASECASE}(a, b)$
  }
  \eIf{$n \emph{\text{ mod }} 2 = 1$}{
    $r \gets \texttt{MUL\_KARATSUBA}(x_{n-2}...x_0, y_{n-2}...y_0)$ \\
    $r \gets \texttt{MUL\_AND\_ADD\_WITH\_OFFSET}(r, x_{n-2}...x_0, y_{n-1}, n-1) $ \\
    $r \gets \texttt{MUL\_AND\_ADD\_WITH\_OFFSET}(r, y, x_{n-1}, n-1) $ \\
  }
  {
    $h \gets \texttt{MUL\_KARATSUBA}(x_{n-1}...x_{n/2}, y_{n-1}...y_{n/2})$ \\
    $t \gets \texttt{MUL\_KARATSUBA}(x_{n-1}...x_{n/2}-x_{n/2-1}...x_{0}, y_{n/2-1}...y_{0}-y_{n-1}...y_{n/2})$ \\
    $l \gets \texttt{MUL\_KARATSUBA}(x_{n/2-1}...x_{0}, y_{n/2-1}...y_{0})$ \\
    $r \gets (2^{2*32*n} + 2^{32*n})*h + 2^{32*n}*t + (2^{32*n}+1)*l$
  }
  \KwRet $r$
}
 \caption{Modular Multiplication}
 \label{alg:mul}
\end{algorithm}
\end{minipage}
\par
}

{\centering
\removelatexerror
\begin{minipage}{\linewidth}
\begin{algorithm}[H]
\scriptsize
\SetAlgoLined
 \KwIn{$x$, $m$, $y$:$y_{n-1}y_{n-2}...y_0$}
 \Indp 
\Indm \KwOut{$x^y \mod m$}
\Indp
\Indm
\SetKwProg{myalg}{function}{}{end}
    \BlankLine
    \BlankLine
\Begin{
  $r \gets 1$ \\
  \For{$i \gets n-1$ \textbf{\emph{to}} $0$ } {
    $r\gets \texttt{SQUARE}(r) \mod m$  \\ 
    \If{$y_i = 1$} {
        $r\gets \texttt{MULTIPLY}(r, x) \mod m$
    }
  }
    \KwRet{$r$} 
  } {}

\caption{Square-and-Multiply Modular Exponentiation}
\label{alg:square-multiply}
\end{algorithm}
\end{minipage}
\par
}

{\centering
\removelatexerror
\begin{minipage}{\linewidth}
\begin{algorithm}[H]
\scriptsize
\SetAlgoLined
 \KwIn{$x$, $m$, $y$:$y_{n-1}y_{n-2}...y_0$}
 \Indp 
\Indm \KwOut{$x^y \mod m$}
\Indp
\Indm
\SetKwProg{myalg}{function}{}{end}
    \BlankLine
    \BlankLine
\Begin{
  $r \gets 1$ \\
  \For{$i \gets n-1$ \textbf{\emph{to}} $0$ } {
    $r\gets \texttt{SQUARE}(r) \mod m$  \\ 
    $r'\gets \texttt{MULTIPLY}(r, x) \mod m$ \\
    \If{$y_i = 1$} {
        $r\gets r'$
    }
  }
    \KwRet{$r$} 
  } {}

 \caption{Square-and-Multiply-always Modular Exponentiation}
 \label{alg:square-multiply-always}
\end{algorithm}
\end{minipage}
\par
}

{\centering
\removelatexerror
\begin{minipage}{\linewidth}
\begin{algorithm}[H]
\scriptsize
\SetAlgoLined
 \KwIn{$x$, $m$, $y$:$w_{n-1}w_{n-2}...w_0$}
 \Indp 
\Indm \KwOut{$x^y \mod m$}
\Indp
\Indm
\SetKwProg{myalg}{function}{}{end}
    \BlankLine
    \BlankLine
\Begin{
  $g[0] \gets x \mod m$ \\
  $s \gets \texttt{SQUARE}(g[0]) \mod m$ \\
  \For{$i \gets 1$ \textbf{\emph{to}} $2^{L-1}-1$ } {
    $g[i] \gets \texttt{MULTIPLY}(g[i-1], s) \mod m$ \\
  }

  \BlankLine
  \BlankLine

  $r \gets 1$ \\
  \For{$i \gets n-1$ \textbf{\emph{to}} $0$ } {
      \For{$j \gets 0$ \textbf{\emph{to}} $l_i-1$ } {
        $r\gets \texttt{SQUARE}(r) \mod m$  \\ 
       }
       \If{$w_i \neq 0$} {
          $r\gets \texttt{MULTIPLY}(r, g[(w_i-1)/2]) \mod m$
        }
  }
    \KwRet{$r$} 
  } {}

 \caption{Sliding Window Modular Exponentiation}
 \label{alg:swe}
\end{algorithm}
\end{minipage}
\par
}

{\centering
\removelatexerror
\begin{minipage}{\linewidth}
\begin{algorithm}[H]
\scriptsize
\SetAlgoLined
\Indp
\Indm
\SetKwFunction{proc}{Scatter}
\SetKwFunction{procg}{Gather}
\SetKwProg{myalg}{function}{}{end}
  $s \gets 8$ \\
  $m \gets 32$ \\
  $b \gets 24$ \\
    \BlankLine
    \BlankLine
  \myalg{\proc{$mem, g[i]$}}{

    \For{$j \gets 0$ \textbf{\emph{to}} $b-1$ }{
      \For{$k \gets 0$ \textbf{\emph{to}} $s-1$ } {
          $mem[s*m*j + i*8 + k] \gets g[i][j*s + k]$  \\ 
      }
    }
  }
  
    \BlankLine
    \BlankLine
  \myalg{\procg{$g[i], mem$}}{
  \For{$j \gets 0$ \textbf{\emph{to}} $b-1$ } {
      \For{$k \gets 0$ \textbf{\emph{to}} $s-1$ } {
        $g[i][j*s+k] \gets mem[s*m*j + i*8 + k]$  \\ 
       }
    }
  }
 \caption{Scatter and Gather method}
 \label{alg:scatter-gather}
\end{algorithm}
\end{minipage}
\par
}

{\centering
\removelatexerror
\begin{minipage}{\linewidth}
\begin{algorithm}[H]
\scriptsize
\SetAlgoLined
\Indp
\Indm
\SetKwFunction{procg}{Gather}
\SetKwProg{myalg}{function}{}{end}
  $s \gets 8$ \\
  $m \gets 32$ \\
  $b \gets 24$ \\
    \BlankLine
    \BlankLine
  \myalg{\procg{$g[i], mem$}}{
  \For{$j \gets 0$ \textbf{\emph{to}} $b-1$ } {
    \For{$l \gets 0$ \textbf{\emph{to}} $m-1$}{
      \For{$k \gets 0$ \textbf{\emph{to}} $s-1$ } {
        $v \gets mem[s*m*j + l*8 + k]$  \\         
        $g[i][j*s+k] \gets g[i][j*s+k] | (v \& (m == l)) $  \\ 
       }
    }
   }
  }
 \caption{Masked Window Gather method}
 \label{alg:mask-gather}
\end{algorithm}
\end{minipage}
\par
}

{\centering
\removelatexerror
\begin{minipage}{\linewidth}
\begin{algorithm}[H]
\scriptsize
\SetAlgoLined
 \KwIn{$P$, $N$:$n_{m-1}n_{m-2}...n_0$}
 \Indp 
\Indm \KwOut{$NP$}
\Indp
\Indm
\SetKwProg{myalg}{function}{}{end}
    \BlankLine
    \BlankLine
\Begin{
  $r \gets 0$ \\
  \For{$i \gets m-1$ \textbf{\emph{to}} $0$ } {
    $r\gets \texttt{PointDouble}(r)$  \\ 
    \If{$n_i = 1$} {
        $r\gets \texttt{PointAdd}(r, P)$
    }
  }
    \KwRet{$r$} 
  } {}

\caption{Double-and-Add Scalar Multiplication}
\label{alg:double-and-add}
\end{algorithm}
\end{minipage}
\par
}

{\centering
\removelatexerror
\begin{minipage}{\linewidth}
\begin{algorithm}[H]
\scriptsize
\SetAlgoLined
 \KwIn{$P$, $N$:$n_{m-1}n_{m-2}...n_0$}
 \Indp 
\Indm \KwOut{$NP$}
\Indp
\Indm
\SetKwProg{myalg}{function}{}{end}
    \BlankLine
    \BlankLine
\Begin{
  $r \gets 0$ \\
  \For{$i \gets m-1$ \textbf{\emph{to}} $0$ } {
    $r\gets \texttt{PointDouble}(r)$  \\ 
    $r'\gets \texttt{PointAdd}(r, P)$ \\
    \If{$n_i = 1$} {
        $r \gets r'$
    }
  }
    \KwRet{$r$} 
  } {}

\caption{Double-and-Add-always Scalar Multiplication}
\label{alg:double-and-add-always}
\end{algorithm}
\end{minipage}
\par
}

{\centering
\removelatexerror
\begin{minipage}{\linewidth}
\begin{algorithm}[H]
\scriptsize
\SetAlgoLined
 \KwIn{$P$, $N$}
 \Indp 
\Indm \KwOut{$NP$}
\Indp
\Indm
\SetKwProg{myalg}{function}{}{end}
    \BlankLine
    \BlankLine
\Begin{

  $i \gets 0$ \\
  \While{$N > 0$}{
    \eIf{$N \emph{\text{ mod }} 2 = 1$}{
      \eIf{$N \emph{\text{ mod }} 2^w \geq 2^{w-1}$}{
        $d_i \gets N \text{ mod } 2^w - 2^w$
      }{
        $d_i \gets N \text{ mod } 2^w$
      }
      $N \gets N - d_i$
    }{
      $d_i \gets 0$
    }
    $N \gets N/2$ \\
    $i \gets i + 1$
  }

  \BlankLine
  \BlankLine

  $g[0] \gets P$ \\
  \For{$j \gets 1$ \textbf{\emph{to}} $2^{w-2}-1$ } {
    $g[j] \gets g[j-1] + P$ \\
  }

  \BlankLine
  \BlankLine

  $r \gets 0$ \\
  \For{$j \gets i-1$ \textbf{\emph{to}} $0$ } {
      $r \gets \texttt{PointDouble}(r)$ \\
      \If{$d_j \neq 0$} {
        \eIf{$d_j > 0$}{
          $r \gets \texttt{PointAdd}(r, g[d_j])$
        }{
          $r \gets \texttt{PointAdd}(r, \texttt{Negative}(g[-d_j]))$
        }
      }
  }
    \KwRet{$r$} 
  } {}

 \caption{Sliding Window Scalar Multiplication}
 \label{alg:naf}
\end{algorithm}
\end{minipage}
\par
}

{\centering
\removelatexerror
\begin{minipage}{\linewidth}
\begin{algorithm}[H]
\scriptsize
\SetAlgoLined
 \KwIn{$x$, $m$}
 \Indp 
\Indm \KwOut{$x^{-1} \text{ mod } m$}
\Indp
\Indm
\SetKwProg{myalg}{function}{}{end}
    \BlankLine
    \BlankLine
\Begin{
  $v \gets m$ \\
  $u \gets x$ \\
  $p \gets 1$ \\
  $q \gets 0$ \\
  \While{$u \neq 0$}{
    \While{\emph{$u \text{ mod } 2 = 0$}}{
      $u \gets u/2$ \\
      \If{\emph{$p \text{ mod } 2 = 1$}}{
        $p \gets p + m$
      }
      $p \gets p /2$
    }
    \While{\emph{$v \text{ mod } 2 = 0$}}{
      $v \gets v/2$ \\
      \If{\emph{$q \text{ mod } 2 = 1$}}{
        $q \gets q + m$
      }
      $q \gets q /2$
    }
    \eIf{$u \geq v$}{
      $u \gets u - v$ \\
      $p \gets p - q$
    }{
      $v \gets v - u$ \\
      $q \gets q - p$
    }
  }
  $r \gets q \text{ mod } m$ \\
    \KwRet{$r$} 
  } {}
\caption{Binary Extended Euclidean Algorithm}
\label{alg:beea}
\end{algorithm}
\end{minipage}
\par
}

{\centering
\removelatexerror
\begin{minipage}{\linewidth}
\begin{algorithm}[H]
\scriptsize
\SetAlgoLined
 \KwIn{$x$, $m$}
 \Indp 
\Indm \KwOut{$x^{-1} \text{ mod } m$}
\Indp
\Indm
\SetKwProg{myalg}{function}{}{end}
    \BlankLine
    \BlankLine
\Begin{
  $v \gets m$ \\
  $u \gets x$ \\
  $p \gets 1$ \\
  $q \gets 0$ \\
  \While{$u \neq 0$}{
    $tmp_1 \gets v \textbf{ div } u$ \\
    $tmp_2 \gets q - tmp_1 * p$ \\
    $tmp_3 \gets v - tmp_1 * u$ \\
    $q \gets p$ \\
    $p \gets tmp_2$ \\
    $v \gets u$ \\
    $u \gets tmp_3$ \\
  }
  \eIf{$q < 0$}{
    $r \gets q + m$ \\
  }{
    $r \gets q$ \\
  }  
    \KwRet{$r$} 
  } {}
\caption{Extended Euclidean Algorithm}
\label{alg:eea}
\end{algorithm}
\end{minipage}
\par
}

{\centering
\removelatexerror
\begin{minipage}{\linewidth}
\begin{algorithm}[H]
\scriptsize
\SetAlgoLined
 \KwIn{$P$, $N$:$n_{m-1}n_{m-2}...n_0$}
 \Indp 
\Indm \KwOut{$NP$}
\Indp
\Indm
\SetKwProg{myalg}{function}{}{end}
    \BlankLine
    \BlankLine
\Begin{
  $r \gets 0$ \\
  $r' \gets P$ \\
  \For{$i \gets m-1$ \textbf{\emph{to}} $0$ } {
    \eIf{$n_i = 0$} {
        $r'\gets \texttt{PointAdd}(r, r')$ \\
        $r\gets \texttt{PointDouble}(r)$ \\
    }{
        $r\gets \texttt{PointAdd}(r, r')$ \\
        $r'\gets \texttt{PointDouble}(r')$ \\
    }
  }
    \KwRet{$r$} 
  } {}

\caption{Montgomery ladder Scalar Multiplication}
\label{alg:montgomery-ladder}
\end{algorithm}
\end{minipage}
\par
}

{\centering
\removelatexerror
\begin{minipage}{\linewidth}
\begin{algorithm}[H]
\scriptsize
\SetAlgoLined
 \KwIn{$P$, $N$:$n_{m-1}n_{m-2}...n_0$}
 \Indp 
\Indm \KwOut{$NP$}
\Indp
\Indm
\SetKwProg{myalg}{function}{}{end}
    \BlankLine
    \BlankLine
\Begin{
  $r \gets 0$ \\
  $r' \gets P$ \\
  \For{$i \gets m-1$ \textbf{\emph{to}} $0$ } {
    $\texttt{ConstSwap}(r, r', n_i)$ \\
    $r'\gets \texttt{PointAdd}(r, r')$ \\
    $r\gets \texttt{PointDouble}(r)$ \\
    $\texttt{ConstSwap}(r, r', n_i)$
  }
    \KwRet{$r$} 
  } {}

\caption{Branchless montgomery ladder Scalar Multiplication}
\label{alg:branchless-montgomery-ladder}
\end{algorithm}
\end{minipage}
\par
}

\subsection{CVSS Calculation (version 2.0)}
\label{sec:cvss-cal}
Equation \ref{eq:base} shows the formula of CVSS 2.0 base metrics. The \emph{Base} score
is determined by two sub-scores: \emph{Exploitability} and \emph{Impact}. 

\emph{Exploitability} measures the difficulty to exploit this vulnerability. It is affected
by three factors: (1) Access Vector (\emph{AV}) reflects the location that the attacker needs
to exploit the vulnerability. A farther location is awarded a higher score.
%The possible value can be local, adjacent network, and remote network. 
(2) Access Complexity (\emph{AC}) embodies the difficulty of the attack required to exploit the 
vulnerability once the adversary gains access to the target system. Lower complexity is awarded a higher score.
%If the adversary requires more privileges, knowledge and information about the target system, or specialized configurations, then the complexity is high, and the score value is low. 
(3) Authentication (\emph{AU}) measures the number of times the adversary
must authenticate to the system in order to exploit the vulnerability. Smaller amount of 
authentications is awarded a higher scores.

\begin{table*}[h!]
\caption{Release history of OpenSSL and GNU Crypto (gray entries contain side-channel patches)}
\label{table:release-history}
\begin{subtable}{0.48\linewidth}
\centering
\resizebox{0.92\linewidth}{!}{
\begin{tabular}{|c|c|c|c|c|c|c|c|c|}
  \hline
\textbf{Date} & \textbf{0.9.6}  & \textbf{0.9.7}  & \textbf{0.9.8}  & \textbf{1.0.0}  & \textbf{1.0.1}  & \textbf{1.0.2}  & \textbf{1.1.0}  & \textbf{1.1.1}  \\
\hline
2000/09/24  & 0.9.6 &   &   &   &   &   &   &   \\
2001/04/05  & 0.9.6a  &   &   &   &   &   &   &   \\
2001/07/09  & \cellcolor{gray}0.9.6b  &   &   &   &   &   &   &   \\
2001/12/21  & 0.9.6c  &   &   &   &   &   &   &   \\
2002/05/08  & 0.9.6d  &   &   &   &   &   &   &   \\
2002/07/30  & 0.9.6e  &   &   &   &   &   &   &   \\
2002/08/08  & 0.9.6f  &   &   &   &   &   &   &   \\
2002/08/09  & 0.9.6g  &   &   &   &   &   &   &   \\
2002/12/05  & 0.9.6h  &   &   &   &   &   &   &   \\
\cline{3-3}
2002/12/31  &   & 0.9.7 &   &   &   &   &   &   \\
2003/02/19  & \cellcolor{gray}0.9.6i  & \cellcolor{gray}0.9.7a  &   &   &   &   &   &   \\
2003/04/10  & \cellcolor{gray}0.9.6j  & \cellcolor{gray}0.9.7b  &   &   &   &   &   &   \\
2003/09/30  & 0.9.6k  & 0.9.7c  &   &   &   &   &   &   \\
2003/11/04  & 0.9.6l  &   &   &   &   &   &   &   \\
2004/03/17  &   & 0.9.7d  &   &   &   &   &   &   \\
2004/05/17  & 0.9.6m  &   &   &   &   &   &   &   \\
\cline{2-2}
2004/10/25  &   & 0.9.7e  &   &   &   &   &   &   \\
2005/03/22  &   & 0.9.7f  &   &   &   &   &   &   \\
2005/04/11  &   & 0.9.7g  &   &   &   &   &   &   \\
\cline{4-4}
2005/07/05  &   &   & \cellcolor{gray}0.9.8 &   &   &   &   &   \\
2005/10/11  &   & \cellcolor{gray}0.9.7h  & 0.9.8a  &   &   &   &   &   \\
2005/10/14  &   & 0.9.7i  &   &   &   &   &   &   \\
2006/05/04  &   & 0.9.7j  & 0.9.8b  &   &   &   &   &   \\
2006/09/05  &   & 0.9.7k  & 0.9.8c  &   &   &   &   &   \\
2006/09/28  &   & 0.9.7l  & 0.9.8d  &   &   &   &   &   \\
\cline{3-3}
2007/02/23  &   &   & 0.9.8e  &   &   &   &   &   \\
2007/10/11  &   &   & \cellcolor{gray}0.9.8f  &   &   &   &   &   \\
2007/10/19  &   &   & 0.9.8g  &   &   &   &   &   \\
2008/05/28  &   &   & 0.9.8h  &   &   &   &   &   \\
2008/09/15  &   &   & 0.9.8i  &   &   &   &   &   \\
2009/01/07  &   &   & 0.9.8j  &   &   &   &   &   \\
2009/05/25  &   &   & 0.9.8k  &   &   &   &   &   \\
2009/11/05  &   &   & 0.9.8l  &   &   &   &   &   \\
2010/02/25  &   &   & 0.9.8m  &   &   &   &   &   \\
2010/03/24  &   &   & 0.9.8n  &   &   &   &   &   \\
\cline{5-5}
2010/03/29  &   &   &   & 1.0.0 &   &   &   &   \\
2010/06/01  &   &   & 0.9.8o  & 1.0.0a  &   &   &   &   \\
2010/11/16  &   &   & 0.9.8p  & 1.0.0b  &   &   &   &   \\
2010/12/02  &   &   & 0.9.8q  & 1.0.0c  &   &   &   &   \\
2011/02/08  &   &   & 0.9.8r  & 1.0.0d  &   &   &   &   \\
2011/09/06  &   &   &   & \cellcolor{gray}1.0.0e  &   &   &   &   \\
2012/01/04  &   &   & \cellcolor{gray}0.9.8s  & \cellcolor{gray}1.0.0f  &   &   &   &   \\
2012/01/18  &   &   & 0.9.8t  & 1.0.0g  &   &   &   &   \\
2012/03/12  &   &   & \cellcolor{gray}0.9.8u  & \cellcolor{gray}1.0.0h  &   &   &   &   \\
\cline{6-6}
2012/03/14  &   &   &   &   & \cellcolor{gray}1.0.1 &   &   &   \\
2012/04/19  &   &   & 0.9.8v  & 1.0.0i  & 1.0.1a  &   &   &   \\
2012/04/23  &   &   & 0.9.8w  &   &   &   &   &   \\
2012/04/26  &   &   &   &   & 1.0.1b  &   &   &   \\
2012/05/10  &   &   & 0.9.8x  & 1.0.0j  & 1.0.1c  &   &   &   \\
2013/02/05  &   &   & \cellcolor{gray}0.9.8y  & \cellcolor{gray}1.0.0k  & \cellcolor{gray}1.0.1d  &   &   &   \\
2013/02/11  &   &   &   &   & 1.0.1e  &   &   &   \\
2014/01/06  &   &   &   & 1.0.0l  & 1.0.1f  &   &   &   \\
2014/04/07  &   &   &   &   & \cellcolor{gray}1.0.1g  &   &   &   \\
2014/06/05  &   &   & \cellcolor{gray}0.9.8za & \cellcolor{gray}1.0.0m  & 1.0.1h  &   &   &   \\
2014/08/06  &   &   & 0.9.8zb & 1.0.0n  & 1.0.1i  &   &   &   \\
2014/10/15  &   &   & \cellcolor{gray}0.9.8zc & \cellcolor{gray}1.0.0o  & \cellcolor{gray}1.0.1j  &   &   &   \\
2015/01/08  &   &   & 0.9.8zd & 1.0.0p  & 1.0.1k  &   &   &   \\
2015/01/15  &   &   & 0.9.8ze & 1.0.0q  & 1.0.1l  &   &   &   \\
\cline{7-7}
2015/01/22  &   &   &   &   &   & 1.0.2 &   &   \\
2015/03/19  &   &   & 0.9.8zf & 1.0.0r  & 1.0.1m  & 1.0.2a  &   &   \\
2015/06/11  &   &   & 0.9.8zg & 1.0.0s  & 1.0.1n  & 1.0.2b  &   &   \\
\cline{5-5}
2015/06/12  &   &   &   &   & 1.0.1o  & 1.0.2c  &   &   \\
2015/07/09  &   &   &   &   & 1.0.1p  & 1.0.2d  &   &   \\
2015/12/03  &   &   & 0.9.8zh &   & 1.0.1q  & 1.0.2e  &   &   \\
\cline{4-4}
2016/01/28  &   &   &   &   & \cellcolor{gray}1.0.1r  & \cellcolor{gray}1.0.2f  &   &   \\
2016/03/01  &   &   &   &   & \cellcolor{gray}1.0.1s  & \cellcolor{gray}1.0.2g  &   &   \\
2016/03/03  &   &   &   &   & \cellcolor{gray}1.0.1t  & \cellcolor{gray}1.0.2h  &   &   \\
2016/08/25  &   &   &   &   &   &   & 1.1.0 &   \\
\cline{8-8}
2016/09/22  &   &   &   &   & \cellcolor{gray}1.0.1u  & \cellcolor{gray}1.0.2i  & 1.1.0a  &   \\
\cline{6-6}
2016/09/26  &   &   &   &   &   & 1.0.2j  & 1.1.0b  &   \\
2016/11/10  &   &   &   &   &   &   & 1.1.0c  &   \\
2017/01/26  &   &   &   &   &   & 1.0.2k  & 1.1.0d  &   \\
2017/02/16  &   &   &   &   &   &   & 1.1.0e  &   \\
2017/05/25  &   &   &   &   &   & 1.0.2l  & 1.1.0f  &   \\
2017/11/02  &   &   &   &   &   & 1.0.2m  & 1.1.0g  &   \\
2017/12/07  &   &   &   &   &   & 1.0.2n  &   &   \\
2018/03/27  &   &   &   &   &   & 1.0.2o  & 1.1.0h  &   \\
2018/08/14  &   &   &   &   &   & \cellcolor{gray}1.0.2p  & \cellcolor{gray}1.1.0i  &   \\
\cline{9-9}
2018/09/11  &   &   &   &   &   &   &   & \cellcolor{gray}1.1.1 \\
2018/11/20  &   &   &   &   &   & \cellcolor{gray}1.0.2q  & \cellcolor{gray}1.1.0j  & \cellcolor{gray}1.1.1a  \\
2019/02/26  &   &   &   &   &   & \cellcolor{gray}1.0.2r  &   & \cellcolor{gray}1.1.1b  \\
\hline
  \end{tabular}
}
\caption{OpenSSL}
\label{table:openssl-release}
\end{subtable}%
\begin{subtable}{0.48\linewidth}
\centering
\resizebox{0.92\linewidth}{!}{
\begin{tabular}{|c|c|c|c|c|c|c|c|c|}
  \hline
\textbf{Date} & \textbf{P1.4.x}  & \textbf{P2.0.x}  & \textbf{P2.1.x}  & \textbf{P2.2.x}  & \textbf{L1.5.x}  & \textbf{L1.6.x}  & \textbf{L1.7.x}  & \textbf{L1.8.x}  \\
\hline
2011/06/29  &   &   &   &   & \cellcolor{gray}1.5.0 &   &   &   \\
%2011/08/04  &   & 2.0.18  &   &   &   &   &   &   \\
%2012/01/30  & 1.4.12  &   &   &   &   &   &   &   \\
%2012/03/27  &   & 2.0.19  &   &   &   &   &   &   \\
2012/12/20  & 1.4.13  &   &   &   &   &   &   &   \\
2013/03/18  &   &   &   &   & 1.5.1 &   &   &   \\
2013/04/18  &   &   &   &   & 1.5.2 &   &   &   \\
2013/05/10  &   & 2.0.20  &   &   &   &   &   &   \\
2013/07/25  & \cellcolor{gray}1.4.14  &   &   &   & \cellcolor{gray}1.5.3 &   &   &   \\
2013/08/19  &   & 2.0.21  &   &   &   &   &   &   \\
2013/10/04  & 1.4.15  & 2.0.22  &   &   &   &   &   &   \\
\cline{7-7}
2013/12/16  &   &   &   &   &   & \cellcolor{gray}1.6.0 &   &   \\
2013/12/18  & \cellcolor{gray}1.4.16  &   &   &   &   &   &   &   \\
2014/01/29  &   &   &   &   &   & 1.6.1 &   &   \\
2014/06/03  &   & 2.0.23  &   &   &   &   &   &   \\
2014/06/23  & 1.4.17  &   &   &   &   &   &   &   \\
2014/06/24  &   & 2.0.24  &   &   &   &   &   &   \\
2014/06/30  & 1.4.18  & 2.0.25  &   &   &   &   &   &   \\
2014/08/07  &   &   &   &   & \cellcolor{gray}1.5.4 &   &   &   \\
2014/08/12  &   & 2.0.26  &   &   &   &   &   &   \\
2014/08/21  &   &   &   &   &   & 1.6.2 &   &   \\
2014/11/06  &   &   & 2.1.0 &   &   &   &   &   \\
2014/12/16  &   &   & 2.1.1 &   &   &   &   &   \\
2015/02/11  &   &   & 2.1.2 &   &   &   &   &   \\
2015/02/18  &   & 2.0.27  &   &   &   &   &   &   \\
2015/02/27  & \cellcolor{gray}1.4.19  &   &   &   &   & \cellcolor{gray}1.6.3 &   &   \\
2015/04/11  &   &   & 2.1.3 &   &   &   &   &   \\
2015/05/12  &   &   & 2.1.4 &   &   &   &   &   \\
2015/06/02  &   & 2.0.28  &   &   &   &   &   &   \\
2015/06/11  &   &   & 2.1.5 &   &   &   &   &   \\
2015/07/01  &   &   & 2.1.6 &   &   &   &   &   \\
2015/08/11  &   &   & 2.1.7 &   &   &   &   &   \\
2015/09/08  &   & 2.0.29  &   &   &   & 1.6.4 &   &   \\
2015/09/10  &   &   & 2.1.8 &   &   &   &   &   \\
2015/10/09  &   &   & 2.1.9 &   &   &   &   &   \\
2015/12/04  &   &   & 2.1.10  &   &   &   &   &   \\
2015/12/20  & 1.4.20  &   &   &   &   &   &   &   \\
2016/01/26  &   &   & 2.1.11  &   &   &   &   &   \\
2016/02/09  &   &   &   &   &   & \cellcolor{gray}1.6.5 &   &   \\
2016/02/18  &   &   &   &   & \cellcolor{gray}1.5.5 &   &   &   \\
2016/03/31  &   & 2.0.30  &   &   &   &   &   &   \\
\cline{8-8}
2016/04/15  &   &   &   &   &   &   & \cellcolor{gray}1.7.0 &   \\
2016/05/04  &   &   & 2.1.12  &   &   &   &   &   \\
2016/06/15  &   &   &   &   &   &   & 1.7.1 &   \\
2016/06/16  &   &   & 2.1.13  &   &   &   &   &   \\
2016/07/14  &   &   & 2.1.14  &   &   &   & 1.7.2 &   \\
2016/08/17  & 1.4.21  &   &   &   & 1.5.6 & 1.6.6 & 1.7.3 &   \\
\cline{6-7}
2016/08/18  &   &   & 2.1.15  &   &   &   &   &   \\
2016/11/18  &   &   & 2.1.16  &   &   &   &   &   \\
2016/12/09  &   &   &   &   &   &   & 1.7.4 &   \\
2016/12/15  &   &   &   &   &   &   & 1.7.5 &   \\
2016/12/20  &   &   & 2.1.17  &   &   &   &   &   \\
2017/01/18  &   &   &   &   &   &   & 1.7.6 &   \\
2017/01/23  &   &   & 2.1.18  &   &   &   &   &   \\
2017/03/01  &   &   & 2.1.19  &   &   &   &   &   \\
2017/04/03  &   &   & 2.1.20  &   &   &   &   &   \\
2017/05/15  &   &   & 2.1.21  &   &   &   &   &   \\
2017/06/02  &   &   &   &   &   &   & 1.7.7 &   \\
2017/06/29  &   &   &   &   &   &   & \cellcolor{gray}1.7.8 &   \\
\cline{9-9}
2017/07/18  &   &   &   &   &   &   &   & \cellcolor{gray}1.8.0 \\
2017/07/19  & \cellcolor{gray}1.4.22  &   &   &   &   &   &   &   \\
2017/07/28  &   &   & 2.1.22  &   &   &   &   &   \\
2017/08/09  &   &   & 2.1.23  &   &   &   &   &   \\
\cline{4-4}
2017/08/27  &   &   &   &   &   &   & \cellcolor{gray}1.7.9 & \cellcolor{gray}1.8.1 \\
2017/08/28  &   &   &   & 2.2.0 &   &   &   &   \\
2017/09/19  &   &   &   & 2.2.1 &   &   &   &   \\
2017/11/07  &   &   &   & 2.2.2 &   &   &   &   \\
2017/11/20  &   &   &   & 2.2.3 &   &   &   &   \\
2017/12/13  &   &   &   &   &   &   &   & 1.8.2 \\
2017/12/20  &   &   &   & 2.2.4 &   &   &   &   \\
2017/12/29  &   & 2.0.31  &   &   &   &   &   &   \\
\cline{3-3}
2018/02/22  &   &   &   & 2.2.5 &   &   &   &   \\
2018/04/09  &   &   &   & 2.2.6 &   &   &   &   \\
2018/05/02  &   &   &   & 2.2.7 &   &   &   &   \\
2018/06/08  &   &   &   & 2.2.8 &   &   &   &   \\
2018/06/11  & 1.4.23  &   &   &   &   &   &   &   \\
2018/06/13  &   &   &   &   &   &   & \cellcolor{gray}1.7.10  & \cellcolor{gray}1.8.3 \\
2018/07/12  &   &   &   & 2.2.9 &   &   &   &   \\
2018/08/30  &   &   &   & 2.2.10  &   &   &   &   \\
2018/10/26  &   &   &   &   &   &   &   & 1.8.4 \\
2018/11/06  &   &   &   & 2.2.11  &   &   &   &   \\
2018/12/14  &   &   &   & 2.2.12  &   &   &   &   \\
2019/02/12  &   &   &   & 2.2.13  &   &   &   &   \\
\hline
  \end{tabular}
}
  \caption{GNU Crypto}
  \label{table:gnupg-release}
  \end{subtable}
\vspace{-15pt}
\end{table*}

\emph{Impact} measures how much damage the vulnerability can incur to the target system. It
is evaluated in terms of three security properties: (1) Confidentiality (\emph{CImpact}) 
refers to the amount of information leaked to the adversary. 
%The possible values can be none (no information leakage), partial (considerable information disclosure), and complete (all information of the target system is leaked). 
(2) Integrity (\emph{IImpact}) refers to the amount of data that the adversary can tamper with. 
%If there is no impact to the integrity of the system, then \texttt{IImpact} is none. If the adversary can control over part of the system's files or files, then \texttt{IImpact} is partial. If the adversary can modify arbitrary data and files on the target system, then \texttt{IImpact} is complete. 
(3) Availability (\emph{AImpact}) measures the loss of access to the system information, 
resources and services. 
%None \texttt{AImpact} means this vulnerability has no availability impact to the system. Partial \texttt{AImpact} means there is reduced performance or interruptions in availability. Complete \texttt{AImpact} means this is a total shutdown of the affected system.
The possible values of the three metrics can be none, partial breach, and complete breach.

\begin{align}
\label{eq:base}
\scriptsize
\begin{split}
& Base = 
\begin{cases}
    0, \qquad \text{if }Impact = 0\\
    (0.6*Impact+0.4*Exploitability-1.5)*1.176, \text{otherwise}
\end{cases} \\
& Exploitability = 20*AV*AC*AU \\
& Impact = 10.41*[1-(1-CImpact)*(1-IImpact)*(1-AImpact)] \\
& AV = 0.395\text{ (local) }/ 0.646\text{ (adjacent network) }/ 1\text{ (network) }\\
& AC = 0.35\text{ (high) }/ 0.61\text{ (medium) }/ 0.71\text{ (low) }\\
& AU = 0.45\text{ (multiple) }/ 0.56\text{ (single) }/ 0.704\text{ (no) }\\
& CImpact = 0\text{ (none) }/ 0.275\text{ (partial) }/ 0.66\text{ (complete) }\\
& IImpact = 0\text{ (none) }/ 0.275\text{ (partial) }/ 0.66\text{ (complete) }\\
& AImpact =  0\text{ (none) }/ 0.275\text{ (partial) }/ 0.66\text{ (complete) }\\
\end{split}
\end{align}

\subsection{Release history of cryptographic libraries}
\label{sec:release-lib}

Table \ref{table:release-history} shows the release history of OpenSSL and GNU Crypto libraries for
the past years. We highlight the released versions containing side-channel patches in gray.

For OpenSSL, we observe that it keeps maintaining about three live branches concurrently throughout
the history. The patches of most vulnerabilities were applied to all live branches at the same time. 
Thus, OpenSSL has good cross-branch patch consistency for side-channel vulnerabilities.

The case of GNU Crypto is more complicated. We ignore GnuTLS as it has too many branches and versions. 
Libgcrypt was previously a module inside GnuPG for cryptographic primitives, but later detached itself 
to become an independent library. As a result, some GnuPG branches (1.4) continued to keep
this module, while others (2.0, 2.1) did not. Also, some implementations of the same
operations in GnuPG and Libgcrypt differed significantly. Thus, side-channel patches
across libraries and branches appeared fairly inconsistent.
